# Supplementary material for: VidToMe: Video Token Merging for Zero-Shot Video Editing
Source: arXiv:2312.10656 source file (2023-12-19)
Supplement: Supplementary file 1 [file X_suppl.tex]

\clearpage
\setcounter{page}{1}
\maketitlesupplementary
\appendix

\section{Video Results}

We present more video editing results in the supplementary video ``Results.mp4", including qualitative comparison with prior r methods and sample editing results on various videos. We summarize our work in another supplementary video ``VidToMe.mp4".

\section{Metrics}
We explain the metrics used in quantitative evaluation, including Interpolation Error and PSNR~\cite{jiang2018super}, Warp Error, Frame CLIP Score, Directional CLIP Score~\cite{gal2022stylegan}, Text CLIP Score, and User Preference Rate. CLIP score metrics are computed in the feature space of the CLIP model~\cite{radford2021learning} for both prompts and frames. Others estimate the optical flow~\cite{teed2020raft} to measure the video continuity.

\noindent \textbf{Warp Error.} Previous works~\cite{lai2018learning} use Warp Err to measure the pixel-level video continuity. It is obtained by warping the edited video frames to adjacent frames by the optical flow estimated on the source video and computing the average mean-squared pixel error between warped and target frames.

\noindent \textbf{Interpolation Error and PSNR.}
Since Warp Error utilizes the source video to estimate the optical flow, it reflects whether the edited video precisely matches the source video in motion.
To measure the video continuity independently, we proposed interpolation-based metrics.
Following video interpolation works~\cite{jiang2018super}, we interpolate a target frame by its previous and next frames and compute the Interpolation Error and PSNR between the interpolated frame and the target frame, where the error is defined as root-mean-squared (RMS) difference between the two frames.

\noindent \textbf{Frame CLIP Score.} Frame CLIP Score is the average CLIP similarity between consecutive frames in the generated video, measuring the video consistency in the CLIP feature space.

\noindent \textbf{Text CLIP Score.} Text CLIP Score is the average CLIP similarity between the edit prompt and the edited frames. However, it is not enough to measure the edit performance with the Text CLIP Score. For example, we can directly generate frames with the edit prompt, omitting the source frames. The resulting frames probably achieve a higher Text CLIP Score than the edited frames, though they are not correlated to source frames.

\noindent \textbf{Directional CLIP Score.} Compared to the consistency between the prompt and frames, it is more important for the editing task to measure the consistency between their changes from source to edit, \ie, whether the change in prompt matches the change in video frames.
Therefore, we use the directional CLIP Score~\cite{gal2022stylegan} to measure the editing effect more precisely, which is the cosine similarity in CLIP space between the difference between the source and edit prompts and the difference between the source and edited frames.

\noindent \textbf{User Preference Rate.} We conduct user studies to evaluate performance in terms of human perception. Users choose their favorite one among the editing results of baselines and our method. Each survey consists of 10 videos, and a total of 27 survey results are collected. User Preference Rate is the average rate of a method preferred by users.

\section{Implementation Details}
Given a source video, we invert video frames into noise latent by DDIM inversion with a text-to-image latent diffusion model, Stable Diffusion~\cite{rombach2022high}. A source prompt is provided as the text condition in inversion. Then we generate the edited video frames with the same diffusion model using an edit prompt as the text condition. Both inversion and generation use the DDIM scheduler with sampling step 50. For the evaluation results, our method keeps video chunk size $B=4$, local and global merging ratio $p=0.9, 0.8$, and a fixed random seed. The hyperparameters are tuned for sample results. The video token merging is applied in the first two downsampling layers and the last two upsampling layers in the diffusion model, right before the self-attention module.

\section{Details of Global Token Merging}
There are two factors related to our global token merging performance, the order to process video chunks and the $src,dst$ assignment in global token merging.

\noindent \textbf{Chunk Processing Order.} In each denoising iteration, video frames are split into consecutive video chunks. The order to process the chunks is related to the global token updating behavior, as global tokens are maintained across chunks. One option is to process the chunks in sequential order. The global tokens are shared among near chunks, boosting the video consistency in consecutive frames. However, distant video frames are still not likely to share tokens as the global tokens are updated gradually. Another choice is to process the chunks in fully random order. The global tokens are randomly shared between chunks independent of the temporal order, promoting global consistency among all video frames. However, tokens from distant frames are less correlated to the current frame, sometimes resulting in quality degradation. We can also combine the two choices to process part of the chunks in random order and the others sequentially, balancing their effect. 

\noindent \textbf{Random Global Token Updating.} In global token merging, local tokens and global tokens are merged to $T_{gm}$. Global tokens are then updated to the local tokens unmerged from $T_{gm}$. Since we use the values of $dst$ tokens as the merged token values, the updated global tokens $T_g^{'}$ are close to the $dst$ tokens. If local tokens ($src$) are merged to the global tokens ($dst$), $T_g^{'}$ consists of most original global tokens and a few new local tokens. Otherwise $T_g^{'}$ has most of its tokens from the current frame chunk. We find that always merging local tokens with global tokens degrades the video quality in some cases since most frames share the same global tokens, overcompressing the video in the feature space. Therefore, we randomly assign $dst, src$ to local and global tokens in the global token merging so that the tokens are properly shared among video chunks. In evaluation, we use random chunk order and assign $dst$ to local tokens with probability $0.5$.

\section{Details of Controlling Methods}
Our method combines an existing controlling method for image editing to maintain the source frame structure. In this work, we apply Plug-and-Play (PnP)~\cite{tumanyan2023plug}, ControlNet~\cite{zhang2023adding}.

\noindent \textbf{PnP.} As PnP injects the self-attention map from source frames to edit frames, their tokens should be aligned. However, token merging may combine different tokens in source and edit frames as the similarity-based matching. To keep the token alignment between source and edit, we enforce their matching map to be the same where the token matching follows the one with a larger similarity in source or edit.

\noindent \textbf{ControlNet.} When combined with ControlNet, the diffusion model may generate over-saturated frames with the DDIM inverted initial noise. We propose to solve the problem by controlled DDIM inversion where the ControlNet is applied in both the inversion and generation process. It ensures the frame can be reconstructed with the source prompt when generated with the same ControlNet as inversion.

\section{Algorithm.} To clarify our method, we provide the pseudocode of the VidToMe algorithm (Algo. \ref{algo:vidtome}). Readers can refer to it for more algorithm details.
\begin{algorithm}[htbp]
  \caption{VidToMe}
  \label{algo:vidtome}
  % \SetKwComment{Comment}{// }
  \SetNoFillComment
  \small
  \SetAlgoLined
  \KwData{$V=(z_1,z_2,\dots,z_{n})$: Source video latents with $n$ frames. $\mathcal{P}_{src}, \mathcal{P}_{edit}$: Source prompt and edit prompt. $\epsilon_{\theta}$: Pretrained text-to-image diffusion model. $G$: Existing controlling method~\cite{zhang2023adding,tumanyan2023plug,rombach2022high}.}
  \KwResult{$V^{*}$: Edited video.}
  \kwHyper{Chunk Size $B$, local and global merging ratio $p_l,p_g$, chunk processing order $O$, merge-to-local probability $q$}
  $c_{src}, c_{edit} \gets$ TextEncoder($\mathcal{P}_{src}, \mathcal{P}_{edit}$)  \tcp*[l]{Encode text prompts to feature space.}
  $V^{T}=(z_1^{T},z_2^{T},\dots,z_{n}^{T}) \gets$ DDIM-Inversion($V, c_{src}, \epsilon_{\theta}$)
   \tcp*[l]{Invert frame into noise latent.}
  \For{$t$:$T\rightarrow 1$}{
    $C \gets$ Chunk($V^{t}, B$) \tcp*[l]{Split video into chunks.}
    $C=(C_1,C_2,\dots,C_m) \gets$ Perm($C, O$) \tcp*[l]{Permute chunks.}
    \For{$i$: $1 \rightarrow m$}{
        $\epsilon_i \gets \epsilon_{\theta}(C_i, t, c_{edit}; G)$  \tcp*[l]{Estimate noise direction using diffusion model with video token merging.}
        
    }
    $\epsilon \gets (\epsilon_1, \epsilon_2,\cdots, \epsilon_{m})$\;
    $V^{t-1} \gets \text{Denoise}(V^{t}, \epsilon, t)$\;
  }
  $V^{*}\gets \text{Decode}(V^{0})$ \tcp*[l]{Decode latents to image.}

  \tcp{Perform video token merging inside the diffusion model.}
  \tcp{Before the self-attention modules.}
        $T_{in} \gets \{T_{in}^{f}\}_{f=0}^{B-1}$\;
        
        \tcp{Local Token Merging}
        $k \gets$ RandInt$(0, B-1)$\;
        $r \gets p_l(B-1)N$\;
        $E_l \gets \text{Match}(\{T_{in}^{f}\}_{f=0,f\neq k}^{B-1}, T_{in}^{k},r))$\;
        $T_{lm} \gets \text{M}(T_{in}, E_l)$\;
        \tcp{Global Token Merging}
        \eIf{$i==1$}{
            $T_g \gets T_{lm}$\;
            $T_{gm} \gets T_{lm}$ \tcp*[l]{Initialize global tokens.}
        }{
            $r \gets p_g(B-1)N$\;
            \eIf{$\text{Rand}(0,1) < q$}{
                $E_g \gets \text{Match}(T_g, T_{lm}, r)$\;
            }{
                $E_g \gets \text{Match}(T_{lm}, T_{g}, r)$\;
            }
            $T_{gm} \gets \text{M}(\{T_{lm}, T_{g}\}, E_g)$\;
            $T_{lm}^{'}, T_{g}^{'} \gets \text{U}(T_{gm}, E_g)$\;
            $T_{g} \gets T_{lm}^{'}$\tcp*[l]{Update global tokens.}
        }
        $T_{o} \gets \text{Self-Attention}(T_{gm})$\;
        \tcp{Token Unmerging}
        $T_{local}, T_{global} \gets \text{U}(T_{o}, E_g)$\;
        $T_{out} \gets \text{U}(T_{local}, E_l)$\;
\end{algorithm}
